# Supplementary material for: Finding Rats in Cats: Detecting Stealthy Attacks using Group Anomaly Detection
Source: arXiv:1905.07273 source file (2019-05-20)
Supplement: Supplementary file 1 [file appendix.tex]

\clearpage
\section{Appendix}
